# Supplementary material for: Estimating Full Path Lengths and Kinetics from Partial Path Transition Interface Sampling Simulations
Source: arXiv:2602.12835 source file (2026-02-13)
Supplement: Supplementary file 1 [file SI.pdf]

# Supporting information: Estimating full path lengths and kinetics from partial path transition interface sampling simulations

Wouter Vervust, Elias Wils, Sina Safaei, Daniel T. Zhang, and An Ghysels

*IBiTech - BioMMedA group, Ghent University,*

*Corneel Heymanslaan 10, entrance 97, 9000 Gent, Belgium*

*Department of Chemistry, Norwegian University of*

*Science and Technology, Trondheim, Norway and*

*Research Institute for Interdisciplinary Science, Okayama University,*

*3-1-1 Tsushima-naka, Okayama, 700-8530, Japan*

**CONTENTS**

I. Additional details of the MSM for REPPTIS S3
A. PPTIS crossing probabilities S3
B. MSM transition matrix S3
C. Limiting states in MSM S4
D. MSM example, $N = 4$ S6

II. Equations for probabilities in MSM network S8
A. Probability to hit state $\beta$ S8
B. Probability to hit state $\beta$ before state $\alpha$ S9
C. Probability to hit state $\beta$ before state $\alpha$, after making at least one step from initial state $\delta$ S11

III. MSM equations for times S12
A. Average time to hit state $\beta$ S12
B. Average time to hit state $\alpha$ or $\beta$ S13
C. Average time to hit states in a set $C$, after leaving state $\delta$ S14

IV. How to solve the matrix equations S15
A. Blocks corresponding to boundary and non-boundary states S15
B. Solving equations for probabilities S16
C. Applied to Eq. 7 (main text) solving for $P_A(\lambda_B|\lambda_A)$ S16
D. Solving MFPT equations S17
E. Applied to Eq. 12 (main text) S18

V. Extra information about 1D potentials simulations S19
A. Simple 1D potentials S19
B. More complex 1D potentials S19
C. Results and error analysis 1D potentials S22

VI. Additional details of KCl dissociation simulations S23
A. MD settings for KCl S23
B. RETIS and REPPTIS simulations of KCl S23

C. Results and error analysis of KCl S24

VII. Additional details of trypsin-benzamidine simulations S24

A. MD settings S24

B. RETIS and REPPTIS simulations S25

C. Results and error analysis S27

D. REPPTIS sampling discussion for trypsin-benzamidine S27

Convergence remarks S27

REPPTIS kinetics in context of prior work S29

Equilibrium MD validation S29

VIII. Assessing REPPTIS convergence S31

References S32

## I. ADDITIONAL DETAILS OF THE MSM FOR REPPTIS

### A. PPTIS crossing probabilities

Prior PPTIS work has consistently used $p_i^{=}$, $p_i^{\pm}$, $p_i^{\mp}$, and $p_i^{\ddagger}$ to denote the local crossing probabilities. They are equivalent to $p_{[i\pm]}^{-1,-1}$, $p_{[i\pm]}^{-1,+1}$, $p_{[i\pm]}^{+1,-1}$, and $p_{[i\pm]}^{+1,+1}$, respectively. The $p_{[i\pm]}^{k,l}$ notation is introduced here to enable general equations, such as the general transition matrix of Eq. S1 below.

### B. MSM transition matrix

The transition probability $P\left(S_i^{k,l} \to S_{i'}^{k',l'}\right)$ is captured by the transition matrix element $M_{ikl,i'k'l'}$, with

$$M_{ikl,i'k'l'} = \begin{cases} p_{[(i+l)\pm]}^{-l,+1}, & i' = i+l, k' = -l, l' = +1 \\ p_{[(i+l)\pm]}^{-l,-1}, & i' = i+l, k' = -l, l' = -1 \\ 0, & \text{elsewhere} \end{cases} \tag{S1}$$

While the indices in Eq. S1 look tedious, it means that the end point $l$ of the segment $S_i^{k,l}$ determines whether the next state is in a higher ensemble $i' = i+1$ ($l = +1$, so end point R) or in a lower ensemble $i' = i-1$ ($l = -1$, so end point L). This explains that the next

visited path ensemble is surely $[i'^{\pm}]$ with $i' = i + l$. Moreover, the end point $l$ determines the starting point of the next segment, so the next starting point is $k' = -l$. The new segment can then have an arbitrary end point, so $l'$ is either $+1$ or $-1$. Interestingly, the elements of $M_{ikl,i'k'l'}$ are independent of the starting point $k$ of the $S_i^{k,l}$ segment, see Eq. S1. This implies that the memory about the initial starting point $k$ is lost. This is indeed implied by the PPTIS ensembles $[i^{\pm}]$ which cover segments with three interface labels but not four labels. Therefore an initial path with labels $(i, k, l)$ will lose information on the label $k$ when a new state is acquired. (The labels $i$ and $l$ survive through the updated labels $i' = i + l$ and $k' = -l$.) Hence, the proposed transition matrix indeed restrains the memory to three labels, in accordance with the PPTIS ensembles.

## C. Limiting states in MSM

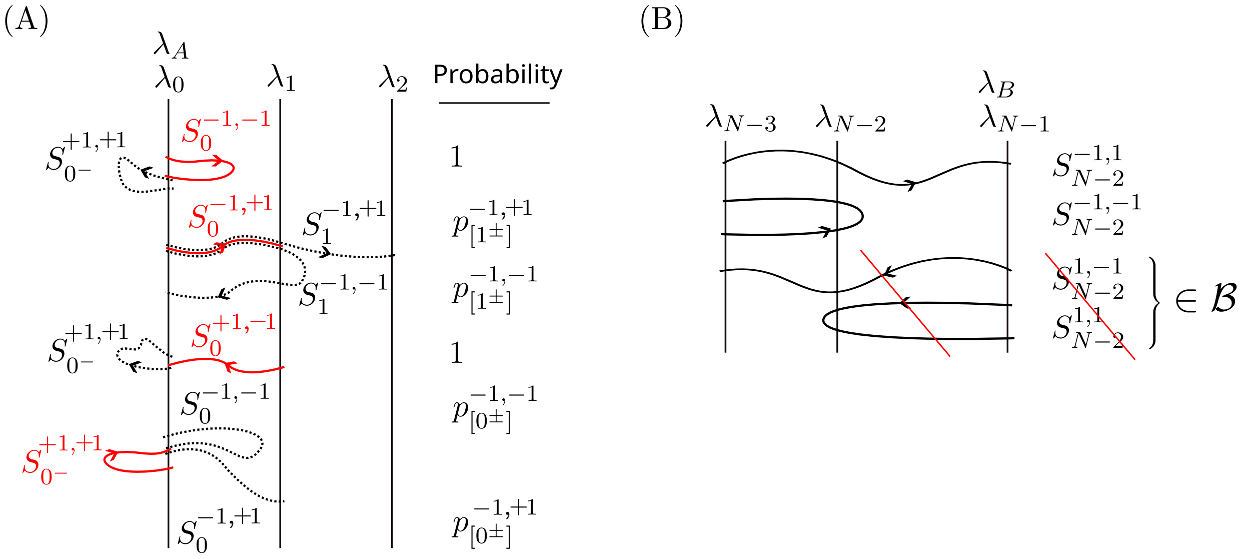


Figure S1: (**A**) The ensembles near $\lambda_A$. The $[0^-]$ ensemble contributes one state and $[0^{\pm}]$ three states to the MSM. All possible transitions and their probabilities are shown. (**B**) The ensemble $[(N-1)^{\pm}]$ near $\lambda_B$. Paths that start from $\lambda_B$ are part of overall state $\mathcal{B}$ [1], and are grouped into $S_{\mathcal{B}}$.

For the interior PPTIS ensembles $[i^{\pm}]$ $i = 1, \ldots, N-2$, there are four states $S_i^{k,l}$ with $k, l \in \{+1, -1\}$, corresponding to the four path types LML, LMR, RML and RMR. The number of states is different for the limiting ensembles associated to $\lambda_0$, $\lambda_{N-1}$, and $\lambda_N$. The

corresponding states and transition probabilities are shown in Figs. S1A-B, and as a graph representation focusing on the limiting ensembles in Fig. S2.

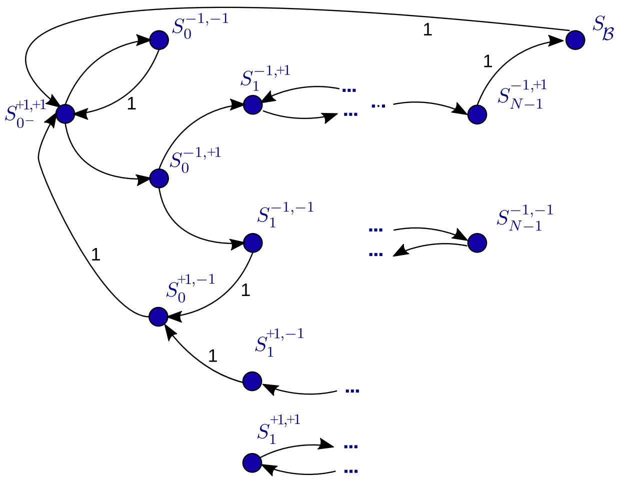


Figure S2: Visualization of the connectivity in the MSM network for the hops between PPTIS segments. Each circle represents a state, while "..." represents multiple states. Transitions with probability 1 are indicated.

For the paths in $[0^-]$, there are only $k = l = +1$ paths (RR type), so this ensemble contributes only one state $S_{0^-}^{+1,+1}$ (Fig. S1A). In path ensemble $[0^\pm]$ , the path types are LL, LR, and RL, so $[0^\pm]$ only contributes three states to the MSM (Fig. S1B).

The RMR and RML segments of $[(N-1)^\pm]$ start at $\lambda_B$, which implies that the trajectory was last in region $B$. These segments are unreachable by any other states of the MSM, and they are combined in a feed-backward state $S_\mathcal{B}$ (Fig. S1B) with $P(S_\mathcal{B} \to S_0^{+1,+1}) = 1$. This essentially means that trajectories that reach state $B$ will eventually return to state $A$, as if recycling boundary conditions were imposed resembling those of weighted ensemble simulations [2]. One could also define $S_\mathcal{B}$ as an absorbing state, which would have no impact on our analysis methodology. With absorbing conditions, however, no equilibrium distribution could be calculated. As of now, we have not yet implemented that.

This brings the number of states to $n_s = 4N - 1$: 1 for $[0^-]$, 3 for $[0^\pm]$ , 2 for $[(N-1)^\pm]$, 1 for $\mathcal{B}$, and 4 for each of the other $N - 2$ ensembles.

### D. MSM example, $N = 4$

As an example, consider a PPTIS simulation with $N = 4$, so 5 interfaces ($\lambda_0$, $\lambda_1$, $\lambda_2$, $\lambda_3$, $\lambda_4$) with $n_s = 4N - 1 = 15$ states. The $15 \times 15$ transition matrix  is given in Eq. S2. The states are ordered first by $i$, then by $k$, and finally by $l$. The sum of each row is equal to 1. The elements that are not shown are equal to zero.

$M =$

| FROM\TO | $S_{0-}^{+1,+1}$ | $S_0^{-1,-1}$ | $S_0^{-1,+1}$ | $S_0^{+1,-1}$ | $S_1^{-1,-1}$ | $S_1^{-1,+1}$ | $S_1^{+1,-1}$ | $S_1^{+1,+1}$ | $S_2^{-1,-1}$ | $S_2^{-1,+1}$ | $S_2^{+1,-1}$ | $S_2^{+1,+1}$ | $S_3^{-1,-1}$ | $S_3^{-1,+1}$ | $S_{\mathcal{B}}$ |
|---|---|---|---|---|---|---|---|---|---|---|---|---|---|---|---|
| $S_{0-}^{+1,+1}$ | | $p_0^{-1,-1}$ | $p_0^{-1,+1}$ | 0 | | | | | | | | | | | |
| $S_0^{-1,-1}$ | 1 | | | | 0 | 0 | 0 | 0 | | | | | | | |
| $S_0^{-1,+1}$ | 0 | | | | $p_1^{-1,-1}$ | $p_1^{-1,+1}$ | 0 | 0 | | | | | | | |
| $S_0^{+1,-1}$ | 1 | | | | 0 | 0 | 0 | 0 | | | | | | | |
| $S_1^{-1,-1}$ | | | | 1 | | | | | 0 | 0 | 0 | 0 | | | |
| $S_1^{-1,+1}$ | | | | 0 | | | | | $p_2^{-1,-1}$ | $p_2^{-1,+1}$ | 0 | 0 | | | |
| $S_1^{+1,-1}$ | | | | 1 | | | | | 0 | 0 | 0 | 0 | | | |
| $S_1^{+1,+1}$ | | | | 0 | | | | | $p_2^{-1,-1}$ | $p_2^{-1,+1}$ | 0 | 0 | | | |
| $S_2^{-1,-1}$ | | | | | 0 | 0 | $p_1^{+1,-1}$ | $p_1^{+1,+1}$ | | | | | 0 | 0 | |
| $S_2^{-1,+1}$ | | | | | 0 | 0 | 0 | 0 | | | | | $p_3^{-1,-1}$ | $p_3^{-1,+1}$ | |
| $S_2^{+1,-1}$ | | | | | 0 | 0 | $p_1^{+1,-1}$ | $p_1^{+1,+1}$ | | | | | 0 | 0 | |
| $S_2^{+1,+1}$ | | | | | 0 | 0 | 0 | 0 | | | | | $p_3^{-1,-1}$ | $p_3^{-1,+1}$ | |
| $S_3^{-1,-1}$ | | | | | | | | | 0 | 0 | $p_2^{+1,-1}$ | $p_2^{+1,+1}$ | | | 0 |
| $S_3^{-1,+1}$ | | | | | | | | | 0 | 0 | 0 | 0 | | | 1 |
| $S_{\mathcal{B}}$ | 1 | | | | | | | | | | | | 0 | 0 | |

(S2)

## II. EQUATIONS FOR PROBABILITIES IN MSM NETWORK

The states in the Markov state model (MSM) are denoted $\alpha$. The transition matrix is denoted $M$ and is of size $n_s \times n_s$ with $n_s$ the number of states in state space. The element $M_{\alpha\beta}$ is de transition probability to jump from state $\alpha$ to state $\beta$. A trajectory can be seen as a series of segments $U_0, U_1, U_2, \ldots$. The state of segment $U_n$ is denoted as $S_n$. The trajectory in the MSM then consists of jumps between states, giving a sequence of states $S_0, S_1, S_2, \ldots$

The correspondence in notations between the main paper and the more general SI is given in Table S1.

| paper | SI | quantity | boundary | matrix eq. | solution |
|---|---|---|---|---|---|
| | $Q_{\delta(\beta)}$ | prob. to hit $\beta$ | $Q_{\beta(\beta)} = 1$ | $Q_{(\beta)} = M' Q_{(\beta)}$ | Eq. S57 |
| $P_\delta$ | $Z_{\delta(\beta)}$ | prob. to hit $\beta$ before $\alpha$ | $Z_{\alpha(\beta)} = 0$, $Z_{\beta(\beta)} = 1$ | $Z_{(\beta)} = M'' Z_{(\beta)}$ | Eq. S57 |
| $P'_\delta$ | $Y_{\delta(\beta)}$ | prob. to hit $\beta$ before $\alpha$, $n \geq 1$ | | $Y_{(\beta)} = M Z_{(\beta)}$ | Eq. S60 |
| | $F_{\delta(\beta)}$ | time to hit $\beta$ | $F_{\beta(\beta)} = 0$ | $F_{(\beta)} = \tau'_{(m2)} + M' F_{(\beta)}$ | Eq. S64 |
| $T_\delta$ | $G_{\delta(C)}$ | time to hit $\alpha$ or $\beta$ | $G_{\alpha(C)} = G_{\beta(C)} = 0$ | $G_{(C)} = \tau''_{(m2)} + M'' G_{(C)}$ | Eq. S64 |
| $T'_\delta$ | $H_{\delta(C)}$ | time to hit $\alpha$ or $\beta$ , $n \geq 1$ | | $H_{(C)} = \tau_{(m2)} + M G_{(C)}$ | Eq. S67 |

Table S1: Overview of probabilities and times computed in the main document (paper) and this document (SI), with indication of the boundary conditions, matrix equation, and equation for the solution. Set $C$ refers to a set of destination states; here $C = \{\alpha, \beta\}$.

### A. Probability to hit state $\beta$

Let us draft equations for the probability $Q$ to hit $\beta$ when the current state is $\delta$,

$$Q_{\delta(\beta)} \equiv P(\exists n \geq 0 : S_n = \beta | S_0 = \delta) \tag{S3}$$

which is a so-called hitting probability. $\beta$ is fixed. When starting from state $\delta = \beta$, we reach $\beta$ with probability 1, because we are already in $\beta$,

$$Q_{\beta(\beta)} = 1 \tag{S4}$$

When starting from $\delta \neq \beta$, we are not yet in $\beta$, and we will have to take at least one step. By conditioning on this first step, the equations for the other hitting probabilities $Q_{\delta(\beta)}$ values

may be constructed,

$$\begin{aligned}
Q_{\delta(\beta)} &= P(\exists n \geq 0 : S_n = \beta | S_0 = \delta) && \text{(S5)}\\
&= P(\exists n \geq 1 : S_n = \beta | S_0 = \delta) && \text{(S6)}\\
&= \sum_{\gamma} M_{\delta\gamma} P(\exists n \geq 1 : S_n = \beta | S_0 = \delta, S_1 = \gamma) && \text{(S7)}\\
&= \sum_{\gamma} M_{\delta\gamma} P(\exists n \geq 1 : S_n = \beta | S_1 = \gamma) && \text{(S8)}\\
&= \sum_{\gamma} M_{\delta\gamma} P(\exists n \geq 0 : S_n = \beta | S_0 = \gamma) && \text{(S9)}\\
&= \sum_{\gamma} M_{\delta\gamma} Q_{\gamma(\beta)} && \text{(S10)}
\end{aligned}$$

The first equality is the definition. The second means that we need to make at least one step because $\delta \neq \beta$. In the third equality, we have conditioned the probability on the outcome of the first step: a transition to any state $\gamma$. In the fourth, the Markovian property removes the dependence on the initial state $S_0 = \delta$. In the fifth, we can see that starting from $S_1$ is equivalent to start over a new chain so we reset the counter of the steps to 0, and in the last equality we recognize the definition of $Q_{\gamma(\beta)}$.

To solve the set of Eqs. S4-S10, an adapted transition matrix $M'$ is constructed where state $\beta$ is made to be absorbing by adapting row $\beta$:

$$M'_{\beta\beta} = 1;\ M'_{\beta\gamma} = 0, \forall \gamma \neq \beta \tag{S11}$$

These elements do not contribute to Eq. S10, so adapting the elements lets us write a compact version of Eq. S10. Indeed, given a specific $\beta$, the equations for the $Q_{(\beta)}$ vector can be summarized, in combination with Eq. S4, by

$$Q_{(\beta)} = M' Q_{(\beta)} \tag{S12}$$

See section IV on how to solve this matrix equation.

### B. Probability to hit state $\beta$ before state $\alpha$

In a next step, we compute the probability $Z$ that a trajectory starting in state $\delta$ can reach state $\beta$ before reaching state $\alpha$,

$$Z_{\delta(\beta)} = P(\exists n \geq 0 : S_n = \beta \,\text{before}\, S_n = \alpha | S_0 = \delta) \tag{S13}$$

which is also a hitting probability. We draft the equations for different starting values $\delta$, where the states $\alpha, \beta$ are fixed.

Starting from $\delta = \alpha$, it is certain that we will not reach $\beta$, because we already reached the $\alpha$ boundary. However, starting from state $\delta = \beta$, we are already in the desired state with certainty, so the probability is 1. This gives the following $Z$ values for these boundaries,

$$Z_{\alpha(\beta)} = 0 \tag{S14}$$

$$Z_{\beta(\beta)} = 1 \tag{S15}$$

When starting from $\delta \neq \beta$ and $\delta \neq \alpha$, we need to take at least one step ($n \geq 1$). By conditioning the probability on this first step, the equations become

$$Z_{\delta(\beta)} = P(\exists n \geq 0 : S_n = \beta \,\text{before}\, S_n = \alpha | S_0 = \delta) \tag{S16}$$

$$= P(\exists n \geq 1 : S_n = \beta \,\text{before}\, S_n = \alpha | S_0 = \delta) \tag{S17}$$

$$= \sum_{\gamma} M_{\delta\gamma} P(\exists n \geq 1 : S_n = \beta \,\text{before}\, S_n = \alpha | S_0 = \delta, S_1 = \gamma) \tag{S18}$$

$$= \sum_{\gamma} M_{\delta\gamma} P(\exists n \geq 1 : S_n = \beta \,\text{before}\, S_n = \alpha | S_1 = \gamma) \tag{S19}$$

$$= \sum_{\gamma} M_{\delta\gamma} P(\exists n \geq 0 : S_n = \beta \,\text{before}\, S_n = \alpha | S_0 = \gamma) \tag{S20}$$

$$= \sum_{\gamma} M_{\delta\gamma} Z_{\gamma(\beta)} \tag{S21}$$

where a similar reasoning is followed as in the derivation of Eq. S10.

These equations can be implemented in practice with an adapted transition matrix $M''$ where the two states $\alpha$ and $\beta$ are both made to be absorbing by adapting their rows,

$$M''_{\alpha\alpha} = 1;\; M''_{\alpha\gamma} = 0, \forall \gamma \neq \alpha \tag{S22}$$

$$M''_{\beta\beta} = 1;\; M''_{\beta\gamma} = 0, \forall \gamma \neq \beta \tag{S23}$$

The equations for the $Z_{(\beta)}$ vector with probabilities to reach the product state from the several states, before reaching the reactant state, can then be summarized as

$$Z_{(\beta)} = M'' Z_{(\beta)} \tag{S24}$$

in combination with Eqs. S14-S15. See again section IV on how to solve this matrix equation.

### C. Probability to hit state $\beta$ before state $\alpha$, after making at least one step from initial state $\delta$

Next, we compute the probability $Y$ that a trajectory that leaves state $\delta$, can reach state $\beta$ before reaching or returning to state $\alpha$,

$$Y_{\delta(\beta)} = P(\exists n \geq 1 : S_n = \beta \,\text{before}\, S_n = \alpha | S_0 = \delta) \tag{S25}$$

For $\delta = \alpha$, this probability is the complement of the *return* probability to state $\alpha$. The number of steps must be at least $n = 1$. It is assumed that $\alpha \neq \beta$.

By conditioning on the first step, the probability to reach $\beta$ before returning to $\alpha$ can be written in terms of the previous $Z$ vectors,

$$\begin{aligned}
Y_{\delta(\beta)} &= P(\exists n \geq 1 : S_n = \beta \,\text{before}\, S_n = \alpha | S_0 = \delta) && \text{(S26)}\\
&= \sum_{\gamma} M_{\delta\gamma} P(\exists n \geq 1 : S_n = \beta \,\text{before}\, S_n = \alpha | S_0 = \delta, S_1 = \gamma) && \text{(S27)}\\
&= \sum_{\gamma} M_{\delta\gamma} P(\exists n \geq 1 : S_n = \beta \,\text{before}\, S_n = \alpha | S_1 = \gamma) && \text{(S28)}\\
&= \sum_{\gamma} M_{\delta\gamma} P(\exists n \geq 0 : S_n = \beta \,\text{before}\, S_n = \alpha | S_0 = \gamma) && \text{(S29)}\\
&= \sum_{\gamma} M_{\delta\gamma} Z_{\gamma(\beta)} && \text{(S30)}
\end{aligned}$$

with similar justifications for the equalities as for the $Q$ or $Z$ vectors in Eqs. S10 or S21, respectively.

This reads in matrix notation as

$$Y_{(\beta)} = M Z_{(\beta)} \tag{S31}$$

By definition, $Y_{\delta(\beta)}$ for $\delta \notin \{\alpha, \beta\}$ is equal to $Z_{\delta(\beta)}$.

## III. MSM EQUATIONS FOR TIMES

The interpretation of $\tau_{(1),\delta}$, $\tau_{(m),\delta}$, $\tau_{(2),\delta}$, and $\tau_{(m2),\delta}$ is explained in the main document. We follow the convention that every additional hop, e.g. from a state $\mu$ to a state $\nu$, will cause an accumulation of extra time of $\tau_{(m2),\mu}$ (independent of $\nu$).

### A. Average time to hit state $\beta$

Assume $F_{\delta(\beta)}$ is the average accumulated time to reach state $\beta$ starting from state $\delta$,

$$F_{\delta(\beta)} = E(t_n^{(\beta)}, n \geq 0 | S_0 = \delta) \tag{S32}$$

where $t_n^{(\beta)}$ denotes the time that the sequence hits state $\beta$ for the first time. When starting in $\delta = \beta$ itself, the sequence $(U_0, U_1, U_2, \ldots)$ is stopped immediately and it consists of only one state $(\beta)$. As there is not hop to any new state yet, the accumulated time for this boundary is zero,

$$F_{\beta(\beta)} = 0 \tag{S33}$$

For $\delta \neq \beta$, at least one step needs to be taken. By conditioning on this step, a recursive relation can be built,

$$\begin{aligned}
F_{\delta(\beta)} &= E(t_n^{(\beta)}, n \geq 0 | S_0 = \delta) & \text{(S34)}\\
&= \sum_\gamma M_{\delta\gamma} E(t_n^{(\beta)} | S_0 = \delta, S_1 = \gamma) & \text{(S35)}\\
&= \sum_\gamma M_{\delta\gamma} (\tau_{(m2),\delta} + E(t_n^{(\beta)} | S_0 = \gamma)) & \text{(S36)}\\
&= \tau_{(m2),\delta} + \sum_\gamma M_{\delta\gamma} F_{\gamma(\beta)} & \text{(S37)}
\end{aligned}$$

In the last equality, the probability conservation $\sum_\gamma M_{\delta\gamma} = 1$ was used, and the definition of $F_{\gamma(\beta)}$ was recognized. An extra time of $\tau_{(m2),\delta}$ is added to the total accumulated time when a hop from state $\delta$ to state $\gamma$ occurs, following the above mentioned convention.

Going into more detail, consider the first state $\delta$, which makes a contribution $\tau_{(m2),\delta}$ (in case there is at least one hop). In some applications of the MFPT equations, this middle part $\tau_{(m),\delta}$ is not relevant, as this lies before the last crossing of $\lambda_i$. Depending on the MFPT that is exactly required, this contribution might need to be deducted, i.e. the desired

MFPT becomes $F_{\delta(\beta)} - \tau_{(m),\delta}$. Now also consider the last state $\beta$, which will not accumulate extra time itself. The first part of the state $\tau_{(1),\beta}$ is implicitly included though, as it is the overlapping segment with the previous state in the sequence. In some applications of the MFPT equations, it might be that also the middle part $\tau_{(m),\beta}$ is required, and then it needs to be added, i.e. the desired MFPT becomes $F_{\delta(\beta)} + \tau_{(m),\beta}$.

Together with Eq. S33, these equations can be written in matrix notation,

$$F_{(\beta)} = \tau'_{(m2)} + M' F_{(\beta)} \tag{S38}$$

Here, $M'$ is the same adapted transition matrix as in Eq. S12 with adsorbing rows for $\beta$. In addition, $\tau'_{(m2)}$ is a column vector that contains the $\tau_{(m2),\delta}$ elements with however a zero entry for the $\beta$ element of this vector.

### B. Average time to hit state $\alpha$ or $\beta$

Next, assume set $A$ contains a set of absorbing states (here, $A = \{\alpha\}$) and set $B$ is a second set with adsorbing states (here, $B = \{\beta\}$). All final destinations of the paths are collected in a set $C = A \cup B$. Assume $A \cap B = \emptyset$. Let us call $\delta$ a general starting state for the path. If a path reached any of the possible destinations in $C$ for the first time after $n$ steps, the accumulated time is denoted as $t_n^C$.

Define $G_{\delta(\beta)}$ as the average accumulated time to reach state $\alpha$ or $\beta$ starting from state $\delta$,

$$G_{\delta(C)} \equiv E(t_n^C, n \geq 0 | S_0 = \delta) \tag{S39}$$

For $\delta \in C$, the boundaries are

$$G_{\delta(C)} = 0 \tag{S40}$$

For $\delta \notin C$, at least one step needs to be taken. By conditioning on this first step, a recursive relation can be built,

$$G_{\delta(C)} = E(t_n^C, n \geq 0 | S_0 = \delta) \tag{S41}$$

$$= \sum_\gamma M_{\delta\gamma} E(t_n^C | S_0 = \delta, S_1 = \gamma) \tag{S42}$$

$$= \sum_\gamma M_{\delta\gamma} (\tau_{(m2),\delta} + E(t_n^C | S_0 = \gamma)) \tag{S43}$$

$$= \tau_{(m2),\delta} + \sum_\gamma M_{\delta\gamma} G_{\gamma(C)} \tag{S44}$$

The reasoning is the same as for the $F$ quantity in Eqs. S33-S37.

Together with Eq. S40, this can be written in matrix notation

$$G_{(C)} = \tau''_{(m2)} + M'' G_{(C)} \tag{S45}$$

where $M''$ is an adapted transition matrix $M$ where all rows corresponding to states in $C$ have been made adsorbing, and $\tau''_{(m2)}$ is the vector with $\tau_{(m2),\delta}$ elements except for the elements $\delta \in C$ that are set to zero.

### C. Average time to hit states in a set $C$, after leaving state $\delta$

The same set $C$ as in the previous subsection is used. Define $H_{\delta(C)}$ as the average accumulated time to reach state $\alpha$ or $\beta$ (more generally: any state in $C$) starting from state $\delta$, given that at least one step has been taken to leave $\delta$,

$$H_{\delta(C)} \equiv E(t_n^C, n \geq 1 | S_0 = \delta) \tag{S46}$$

Conditioning on this first step gives an expected stopping time $H_{\delta(C)}$,

$$H_{\delta(C)} = E(t_n^C, n \geq 1 | S_0 = \delta) \tag{S47}$$

$$= \sum_\gamma M_{\delta\gamma} E(t_n^C, n \geq 1 | S_0 = \delta, S_1 = \gamma) \tag{S48}$$

$$= \sum_\gamma M_{\delta\gamma} (\tau_{(m2),\delta} + E(t_n^C, n \geq 0 | S_0 = \gamma)) \tag{S49}$$

$$= \tau_{(m2),\delta} + \sum_\gamma M_{\delta\gamma} G_{\gamma(C)} \tag{S50}$$

using a similar reasoning as for deriving Eq. S37.

In matrix notation, these equations become

$$H_{(C)} = \tau_{(m2)} + M G_{(C)} \tag{S51}$$

with $M$ the (unmodified) transition matrix, $G_{(C)}$ the previously computed vector of Eq. S45, and $\tau_{(m2)}$ is the vector with $\tau_{(m2),\delta}$ elements.

In case the set $C$ only contains one state $\alpha$, then for $\delta = \alpha$, the element $H_{\alpha(C)}$ has the interpretation of a return time to state $\alpha$. For $\delta \notin C$, the elements relate to the previously computed $G_{(\beta)}$ vector, i.e. $H_{\delta(C)} = G_{\delta(C)}$, $\forall \delta \neq \alpha$.

## IV. HOW TO SOLVE THE MATRIX EQUATIONS

### A. Blocks corresponding to boundary and non-boundary states

In order to solve the matrix equations for the vector $Q_{(\beta)}$, $Z_{(\beta)}$, etc., the transition matrix $M$ is reorganized to put the absorbing rows for $\beta$ (for $\alpha$ and $\beta$) to the top and corresponding columns to the left of the matrix. For generality, assume the set $C$ contains all $n_b$ boundary states, and $n_s$ is the total number of states. The number of non-boundary states is $n_n = n_s - n_b$. The reorganized matrix has four blocks,

$$M = \begin{pmatrix} M_{bb} & M_{bn} \\ M_{nb} & M_{nn} \end{pmatrix} \tag{S52}$$

corresponding to the boundary (b) and non-boundary (n) states. The diagonal block $M_{bb}$ has dimension $n_b \times n_b$, and the diagonal block $M_{nn}$ has dimension $n_n \times n_n$. The off-diagonal block $M_{nb}$ has dimension $n_n \times n_b$, while $M_{bn}$ has dimension $n_b \times n_n$.

Another matrix that is needed, is the adapted transition matrix $M'$ where the $M_{bb}$ and $M_{bn}$ block in the transition matrix $M$ are set to adsorbing rows, thus $M_{bb} \to 1_b$ and $M_{bn} \to 0$, where $1_b$ is an identity matrix of equal size as $M_{bb}$,

$$M' = \begin{pmatrix} 1_b & 0 \\ M_{nb} & M_{nn} \end{pmatrix} \tag{S53}$$

The adapted matrix $M''$ (e.g. in Eq. S24 for $Z_{(\beta)}$) is similar to $M'$, but the selected states in $C$ differ.

Similarly to $M$ and $M'$, vectors can also be reordered and split up in blocks corresponding to boundary (b) and non-boundary (n) blocks. For instance, a vector $q$ of dimension $n_s \times 1$ can reordered and then be split up in a part $q_b$ of dimension $n_b \times 1$ corresponding to the boundary states in $C$ and a part $q_n$ of dimension $n_n \times 1$ for the remainder of the $q$ vector corresponding to the non-boundary states,

$$q = \begin{pmatrix} q_b \\ q_n \end{pmatrix} \tag{S54}$$

### B. Solving equations for probabilities

The matrix equations for $Q$ or $Z$ are of the shape $q = M'q$. The equations $q = M'q$ read in block diagonal matrix form,

$$\begin{pmatrix} q_b \\ q_n \end{pmatrix} = \begin{pmatrix} 1_b & 0 \\ M_{nb} & M_{nn} \end{pmatrix} \begin{pmatrix} q_b \\ q_n \end{pmatrix} \tag{S55}$$

where $q_b = q_b^0$ are the known boundary values that should be taken into account. The matrix equation is then equivalent to

$$\begin{cases} q_b &= q_b^0 \\ q_n &= M_{nb} q_b + M_{nn} q_n \end{cases} \tag{S56}$$

with solution

$$\begin{cases} q_b &= q_b^0 \\ q_n &= (1_n - M_{nn})^{-1} M_{nb} q_b^0 \end{cases} \tag{S57}$$

Next, a matrix equation of the shape $y = Mq$ can be computed, for instance for the computation of $Y$ in Eq. S30. The vector $y$ becomes

$$\begin{pmatrix} y_b \\ y_n \end{pmatrix} = \begin{pmatrix} M_{bb} & M_{bn} \\ M_{nb} & M_{nn} \end{pmatrix} \begin{pmatrix} q_b \\ q_n \end{pmatrix} \tag{S58}$$

The matrix equation is equivalent to

$$\begin{cases} y_b &= M_{bb} q_b + M_{bn} q_n \\ y_n &= M_{nb} q_b + M_{nn} q_n = q_n \end{cases} \tag{S59}$$

and thus

$$\begin{cases} y_b &= M_{bb} q_b^0 + M_{bn} (1_n - M_{nn})^{-1} M_{nb} q_b^0 \\ y_n &= q_n = (1_n - M_{nn})^{-1} M_{nb} q_b^0 \end{cases} \tag{S60}$$

### C. Applied to Eq. 7 (main text) solving for $P_A(\lambda_B|\lambda_A)$

The first step is to construct $M$ of size $n_s \times n_s$ and to compute the $P$ vector from Eqs. 4-7 in the main text, followed by the computation of $P'_\alpha$ from Eq. 7 in the main text. Reshuffle the order of the states in the matrix $M$, with the boundary $\alpha$ and $\beta$ as the top rows and first columns, and the non-boundary states below. There are $n_\mathrm{b} = 2$ boundary states and

$n_{\mathrm{n}} = n_s - 2$ non-boundary states ($n_{\mathrm{b}} + n_{\mathrm{n}} = n_s$). Define the corresponding boundary (b) and non-boundary (n) subblocks in this reshuffled matrix as $M_{\mathrm{bb}}$, $M_{\mathrm{bn}}$, $M_{\mathrm{nb}}$, and $M_{\mathrm{nn}}$ of size $2 \times 2$, $2 \times n_{\mathrm{n}}$, $n_{\mathrm{n}} \times 2$, and $n_{\mathrm{n}} \times n_{\mathrm{n}}$, respectively. Similarly, reshuffle the elements in the $P$ vector, and define subblocks $P_{\mathrm{n}}$ and $P_{\mathrm{b}}$ of dimension $n_{\mathrm{n}} \times 1$ and $2 \times 1$, respectively; hence $P_{\mathrm{b}} = [P_\alpha, P_\beta]^T = [0, 1]^T$. Perform the same reshuffling in $P'$ and define the subblocks $P'_{\mathrm{n}}$ and $P'_{\mathrm{b}} = \left[P'_\alpha, P'_\beta\right]^T$. With $1_{\mathrm{n}}$ the identity matrix of equal size as $M_{\mathrm{nn}}$, compute the $2 \times 1$ matrix $P'_{\mathrm{b}}$

$$P'_{\mathrm{b}} = M_{\mathrm{bb}} P_{\mathrm{b}} + M_{\mathrm{bn}} (1_{\mathrm{n}} - M_{\mathrm{nn}})^{-1} M_{\mathrm{nb}} P_{\mathrm{b}} \tag{S61}$$

Here, $P_A(\lambda_B|\lambda_A)$ is the first element $P'_\alpha$ of this matrix, whilst the second element $P'_\beta$ is equal to 0.

### D. Solving MFPT equations

The matrix equations for $F$ and $G$ are of the shape $u = \tau' + M'u$. Introducing a decomposition for $\tau'$ into $\tau'_b = 0$ and $\tau'_n$, the matrix equation $u = \tau + M'u$ reads

$$\begin{pmatrix} u_b \\ u_n \end{pmatrix} = \begin{pmatrix} 0 \\ \tau_n \end{pmatrix} + \begin{pmatrix} 1_b & 0 \\ M_{nb} & M_{nn} \end{pmatrix} \begin{pmatrix} u_b \\ u_n \end{pmatrix} \tag{S62}$$

while the known boundary conditions $u_b = u_b^0$ also need to be respected. The matrix equation is then equivalent to

$$\begin{cases} u_b &= u_b^0 \\ u_n &= \tau_n + M_{nb} u_b + M_{nn} u_n \end{cases} \tag{S63}$$

with solution

$$\begin{cases} u_b &= u_b^0 \\ u_n &= (1_n - M_{nn})^{-1} \left(\tau_n + M_{nb} u_b^0\right) \end{cases} \tag{S64}$$

Next, a matrix equation in the shape $v = \tau + Mu$ can be computed, e.g. for the time vector $H$. The vector $v$ is equal to

$$\begin{pmatrix} v_b \\ v_n \end{pmatrix} = \begin{pmatrix} \tau_b \\ \tau_n \end{pmatrix} + \begin{pmatrix} M_{bb} & M_{bn} \\ M_{nb} & M_{nn} \end{pmatrix} \begin{pmatrix} u_b \\ u_n \end{pmatrix} \tag{S65}$$

The matrix equation is equivalent to

$$\begin{cases} v_b &= \tau_b + M_{bb} u_b + M_{bn} u_n \\ v_n &= \tau_n + M_{nb} u_b + M_{nn} u_n = u_n \end{cases} \tag{S66}$$

and thus

$$\begin{cases} v_b &= \tau_b + M_{bb} u_b^0 + M_{bn} (1_n - M_{nn})^{-1} \left(\tau_n + M_{nb} u_b^0\right) \\ v_n &= u_n = (1_n - M_{nn})^{-1} \left(\tau_n + M_{nb} u_b^0\right) \end{cases} \tag{S67}$$

Specifically for $F$, $G$, and $H$ in this document, we have here $u_b = u_b^0 = 0$, which simplifies the time vectors $u$ and $v$ to

$$\begin{cases} u_b &= 0 \\ u_n = v_n &= (1_n - M_{nn})^{-1} \tau_n \\ v_b &= \tau_b + M_{bn} (1_n - M_{nn})^{-1} \tau_n \end{cases} \tag{S68}$$

### E. Applied to Eq. 12 (main text)

Similarly as for the crossing probability in Eq. S61, the first step is to construct $M$ (assume of size $n_s \times n_s$). There are $n_{\mathrm{b}}$ boundary states (# elements in set C) and $n_{\mathrm{n}}$ non-boundary states (with $n_{\mathrm{b}} + n_{\mathrm{n}} = n_s$). Explicitly, reshuffle again the $M$ matrix such that the boundary (b) and non-boundary (n) subblocks can be extracted, i.e. $M_{\mathrm{bb}}$, $M_{\mathrm{bn}}$, $M_{\mathrm{nb}}$, and $M_{\mathrm{nn}}$. Similarly, reshuffle the $\tau_{(m2)}$ vector and extract the subblocks $\tau_{(m2),\mathrm{b}}$ and $\tau_{(m2),\mathrm{n}}$ of size $n_{\mathrm{b}} \times 1$ and $n_{\mathrm{n}} \times 1$, respectively. Also reshuffle vector $T$ into blocks $T_{\mathrm{n}}$ and $T_{\mathrm{b}}$ and reshuffle vector $T'$ into blocks $T'_{\mathrm{n}}$ and $T'_{\mathrm{b}} = [T'_\alpha, T'_\beta]^T$. Whereas the $T_{\mathrm{b}}$ vector is a zero vector by construction (boundaries Eq. 11 in the main text), all other times can be computed from the (shuffled) $M$ and $\tau_{(m2)}$ blocks using matrix operations,

$$T'_{\mathrm{n}} = T_{\mathrm{n}} = (1_{\mathrm{n}} - M_{\mathrm{nn}})^{-1} \tau_{(m2),\mathrm{n}} \tag{S69}$$

$$T'_{\mathrm{b}} = M_{\mathrm{bn}} (1_{\mathrm{n}} - M_{\mathrm{nn}})^{-1} \tau_{(m2),\mathrm{n}} + \tau_{(m2),\mathrm{b}} \tag{S70}$$

where the $T'_{\mathrm{b}}$ contains the interesting times $T'_\alpha$ and $T'_\beta$ to reach destinations in $C$, given that at least one step is taken.

## V. EXTRA INFORMATION ABOUT 1D POTENTIALS SIMULATIONS

### A. Simple 1D potentials

The four simple potentials are: 'flat' (no bumps), '2 bumps', '3 bumps', and '2 dips' (inverted bumps). They are visualized with their respective interfaces in Fig. 6A.

The potential is defined as

$$V(x) = \begin{cases} \frac{1}{2}V_0\left(\cos\frac{\pi(x-a(N_b+1))}{a}+1\right), & |x| \leq N_b\, a \\ 0, & N_b\, a < |x| \leq b \\ \frac{1}{2}k_{\text{harm}}(|x|-b)^2. & |x| > b \end{cases} \tag{S71}$$

which makes the force on $x$ a continuous function for all $x$. Reduced units were used to simplify the calculations, meaning the mass $m$, temperature $T$ and Boltzmann constant $k_B$ are normalized to unity [3]. The parameters in the simulations are $a = 0.1$, $b = N_b\, a + 0.1$, and the strength of the harmonic walls is $k_{\text{harm}} = 100$. The potential height is set to $V_0 = 0$ for the flat potential, $V_0 = 1$ for bumps, or $V_0 = -1$ for dips. The parameter $N_b$ is the number of cosine-shaped bumps with period $2a$, with the exception of the flat potential, where it is the width of the region between state $A$ and state $B$. It is set by $N_b = 3$ for the flat potential, $N_b = 2$ for '2 bumps' and '2 dips', and $N_b = 3$ for '3 bumps'. The particle dynamics were Brownian, Langevin, or Newtonian, integrated with timestep $\Delta t = 2 \cdot 10^{-4}$. The dynamics parameters were set according to Ref. [1], with a relatively low friction coefficient $\gamma = 5$ when using Langevin dynamics. The subcycle setting is put to 1, meaning the engine writes out every integrated timestep to the RETIS algorithm.

The number of interfaces was chosen to be $2N_b + 1$, proportional to the number of bumps $N_b$. The interfaces were uniformly spaced with a distance $a$ between them, letting them correspond with the extrema of the cosine bumps/dips potentials. For the flat potential, five equally-spaced interfaces were used.

### B. More complex 1D potentials

Additionally, two more complex 1D potentials were studied; one with three bumps of different height ('metastable bump'), and one containing a potential well ('rugged dip'), with added modulation to simulate smaller metastable states.

| Potential | Dynamics | $P_A(\lambda_B\|\lambda_A)$ $(\times 10^{-2})$ | | $\tau_{[0^+]}$ [#ph] | | $\tau_{[0^\pm]}$ [#ph] | $f_A$ [1/time, red.] | | $k_{\mathrm{AB}}$ [1/time, red.] | |
|---|---|---|---|---|---|---|---|---|---|---|
| | | RETIS | REPPTIS* | RETIS | REPPTIS* | REPPTIS | RETIS | REPPTIS* | RETIS | REPPTIS* |
| flat | Brownian | 2.62 (7%) | 2.55 (8%) | 56.5 (2%) | 52.7 (6%) | 16.6 (1%) | 41.5 (5%) | 42.7 (3%) | 1.09 (9%) | 1.09 (8%) |
| | Langevin | 51.6 (2%) | 50.7 (1%) | 2510. (0.5%) | 2550. (0.5%) | 604. (0.5%) | 0.926 (2%) | 0.921 (0.4%) | 0.478 (2%) | 0.467 (1%) |
| | Newtonian | 100. (0%) | 100. (0%) | 2531. (1%) | 2495. (2%) | 620. (1%) | 0.946 (1%) | 0.938 (1%) | 0.946 (1%) | 0.938 (1%) |
| 2 bumps | Brownian | 1.50 (8%) | 1.48 (5%) | 33.0 (2%) | 34.5 (3%) | 14.3 (1%) | 52.0 (5%) | 51.9 (3%) | 0.779 (9%) | 0.767 (4%) |
| | Langevin | 23.7 (3%) | 22.7 (2%) | 1581. (1%) | 1589. (1%) | 601. (0.4%) | 1.13 (1%) | 1.13 (1%) | 0.268 (3%) | 0.256 (2%) |
| 3 bumps | Brownian | 1.03 (9%) | 1.03 (6%) | 62.7 (3%) | 52.1 (5%) | 15.9 (1%) | 40.5 (7%) | 45.6 (5%) | 0.415 (11%) | 0.470 (5%) |
| | Langevin | 18.9 (3%) | 17.5 (2%) | 2468. (1%) | 2354. (2%) | 593. (0.4%) | 0.944 (1%) | 0.962 (1%) | 0.179 (3%) | 0.168 (2%) |
| 2 dips | Brownian | 4.00 (8%) | 4.00 (5%) | 97.0 (2%) | 94.0 (5%) | 18.8 (1%) | 32.9 (6%) | 32.1 (5%) | 1.313 (10%) | 1.268 (4%) |
| | Langevin | 53.4 (1%) | 52.5 (2%) | 4498. (1%) | 4505. (2%) | 426. (0.4%) | 0.685 (1%) | 0.684 (1%) | 0.366 (2%) | 0.359 (1%) |
| metastable bump | Brownian | 1.09 (9%) | 1.01 (4%) | 56.6 (3%) | 49.3 (3%) | 14.2 (1%) | 43.2 (6%) | 43.3 (3%) | 0.472 (10%) | 0.437 (4%) |
| | ↪ fine | 1.01 (5%) | 1.05 (10%) | 53.2 (3%) | 48.5 (5%) | 5.12 (1%) | 46.0 (5%) | 45.5 (6%) | 0.463 (7%) | 0.481 (9%) |
| | ↪ shifted | 0.95 (6%) | 0.96 (4%) | 49.6 (3%) | 50.0 (3%) | 11.1 (1%) | 46.2 (5%) | 45.9 (4%) | 0.438 (8%) | 0.440 (4%) |
| | Langevin | 21.2 (2%) | 20.3 (2%) | 2277. (1%) | 2244. (1%) | 610. (0.4%) | 0.971 (1%) | 0.982 (1%) | 0.206 (2%) | 0.199 (2%) |
| | ↪ fine | 20.3 (2%) | 17.0 (3%) | 2263. (1%) | 2264. (1%) | 219. (1%) | 0.983 (1%) | 0.973 (1%) | 0.200 (3%) | 0.165 (3%) |
| | ↪ shifted | 20.5 (2%) | 20.3 (2%) | 2294. (1%) | 2250. (1%) | 455. (0.5%) | 0.977 (1%) | 0.988 (1%) | 0.200 (3%) | 0.201 (3%) |
| rugged dip | Brownian | 2.49 (8%) | 2.48 (5%) | 127.7 (3%) | 135.1 (5%) | 16.1 (1%) | 28.4 (7%) | 27.9 (3%) | 0.709 (11%) | 0.681 (3%) |
| | Langevin | 41.9 (2%) | 39.5 (2%) | 6112. (1%) | 6064. (1%) | 572.3 (0.4%) | 0.602 (2%) | 0.605 (1%) | 0.252 (2%) | 0.239 (2%) |

Table S2: Results of the 1D potential RETIS and REPPTIS simulations after 30 000 cycles. Columns labeled with REPPTIS* were obtained by applying the MSM framework to REPPTIS quantities. Crossing probability $P_A(\lambda_B|\lambda_A)$: REPPTIS values computed with recursive scheme (not shown) [4] are indiscernible from our new MSM-formula in Eq. 7. Average path length $\tau_{[0^+]}$ (# phasepoints) according to RETIS and MSM-based REPPTIS value of Eq. 13. Average path length $\tau_{[0^\pm]}$ from REPPTIS. Flux $f_A$ and rate $k_{\mathrm{AB}}$ (reduced units) computed using RETIS and MSM-based REPPTIS (Eq. 14 and Eq. 20). Relative standard error is given between brackets, as estimated from block averaging (see main text). These errors are shown as whole-number percentages unless below 0.5%, in which case they are shown with one decimal.

The analytical expression for the metastable cosine-shaped bump ('metastable bump') with smaller bumps on top, is

$$V(x) = \begin{cases} \frac{1}{2}k_{\text{harm}}(|x|-b)^2 & x < -b \\ 0, & -b \le x \le -(2a+w) \\ \frac{h}{2}\left(\cos\frac{2\pi(x+2a)}{w}+1\right), & -(2a+w) < x \le -2a \\ h+\frac{1}{2}V_0\left(\cos\frac{\pi x}{a}-1\right), & -2a < x \le -a \\ h+(V_1-V_0)+\frac{1}{2}V_1\left(\cos\frac{\pi x}{a}-1\right), & -a < x \le a \\ h+\frac{1}{2}(V_2-(V_1-V_0))\left(\cos\frac{\pi x}{a}-1\right), & a < x \le 2a \\ d\cdot h+(1-d)\frac{h}{2}\left(\cos\frac{2\pi(x-2a)}{w}+1\right), & 2a < x \le 2a+w \\ d\cdot h, & 2a+w < x \le b \\ d\cdot h+\frac{1}{2}k_{\text{harm}}(|x|-b)^2. & x > b \end{cases} \tag{S72}$$

Just like with the simple cosine bumps in Eq. S71, the force is continuous over the full domain. The parameters $h$ and $w$ refer to the main barrier height and width respectively, while $d$ is the fraction of the barrier height that determines the potential energy at state $B$. The energies $V_0$, $V_1$ and $V_2$ are the amplitudes of the 3 asymmetric cosine bumps present. Other parameters have the same meaning as those of the simpler potentials above. In the calculations, the parameters were set to $h = 0.8$, $w = 0.1$, $d = 0.2$, $V_0 = 0.5$, $V_1 = 0.8$, $V_2 = 0.75$, $k_{\text{harm}} = 100$, $a = 0.1$, and $b = 2a + w + 0.1$.

Three choices for the interfaces are considered for the metastable bump potential.

1. For the first choice, the 7 interfaces are equally-spaced between $\lambda = -0.3$ and 0.3 and are located at $[-0.3, -0.2, -0.1, 0., 0.1, 0.2, 0.3]$.

2. For the second choice, the 19 interfaces forme a finer grid and are located at

   $$[-0.1, -0.066, -0.033, 0., 0.033, 0.066,$$
   $$0.1, 0.133, 0.166, 0.2, 0.233, 0.266,$$
   $$0.3, 0.333, 0.366, 0.4, 0.433, 0.466, 0.5].$$

3. In the third choice, 7 interfaces are located at $[-0.3, -0.23, -0.14, -0.01, 0.06, 0.24, 0.3]$, meaning that the 5 inner interfaces, of the original 7 equally-spaced interfaces between $\lambda = -0.3$ and 0.3, are shifted compared to the first choice.

The rugged cosine-shaped well ('rugged dip') has the following piecewise analytical expression,

$$V(x) = \begin{cases} \frac{1}{2}k_{\mathrm{harm}}(|x|-b)^2 & x < -b \\ 0, & -b \leq x \leq -(a+w) \\ \frac{h}{2}\left(1-\cos\frac{\pi(x-a+w)}{w}\right), & -(a+w) < x \leq -a \\ h + \frac{V_0}{2}\left(\cos\frac{\pi(x-a)}{a}-1\right) - \left(V_m \cdot \cos\frac{2\pi x}{T_m}\right)\cdot\left(1-\cos\frac{\pi(x-a)}{a}\right), & -a < x \leq a \\ d\cdot h + (1-d)\frac{h}{2}\left(1-\cos\frac{\pi(x-a+w)}{w}\right), & a < x \leq a+w \\ d\cdot h, & a+w < x \leq b \\ d\cdot h + \frac{1}{2}k_{\mathrm{harm}}(|x|-b)^2. & x > b \end{cases} \tag{S73}$$

The potential consists of a starting slope the particle needs to cross, after which a large well is present, and finally the particle again rolls down a slope to reach state $B$. The large well is modulated by smaller and higher frequency cosine waves. The force is again continuous over the full domain. Here $2a$ is the period of the big cosine-shaped well, while $h$ and $w$ are the height and width of the starting and ending slope that the particle needs to cross. The modulation of the well is determined by the modulation amplitude $V_m$ and period $T_m$. The rest of the variables have the same meaning as described before. For this application the parameter values were $a = 0.25$, $b = a + w + 0.1$, $h = 0.15$, $w = 0.05$, $V_0 = 1.2$, $V_m = 0.12$, $T_m = 0.06$, $d = 0$, and $k_{\mathrm{harm}} = 100$.

For these potentials, reduced units are used (PyRETIS 3) [3], using timestep $\Delta t = 2\cdot 10^{-4}$ and subcycle 1.

### C. Results and error analysis 1D potentials

The numerical results of the RETIS and MSM-corrected values are listed in Table S2, along with the REPPTIS-native $\tau_{[0\pm]}$ for comparison.

Error analysis was performed using the recursive block error analysis implementation [3], as calculating statistical errors in RETIS and REPPTIS simulations is challenging due to complex correlations between path ensembles, and the standard block averaging implementation struggles with issues such as path swapping and varying trajectory counts [3]. The

recursive block error algorithm starts by computing the running estimate of a key property, such as crossing probability or average path length, as a function of MC cycles. The final value of the running estimates is the best estimate of the property. The algorithm then computes the block average for a series of block sizes. The minimum number of blocks was set to five, ensuring a sufficient number of blocks for averaging, and thus the block size varied here from one to 600 MC cycles. For each block size, the standard error over the blocks was computed, and the relative error was obtained by normalizing against the best estimate. In the relative error versus block size plot, the second half of the relative error values was then averaged to determine the final standard error estimate.

## VI. ADDITIONAL DETAILS OF KCL DISSOCIATION SIMULATIONS

### A. MD settings for KCl

Utilizing GROMACS version 2024.4, the simulated system consists of 1 ion pair of KCl solvated in a cubic box of 508 water molecules. The interactions were modelled with the CHARMM36m modified TIP3P water model [5] and the ion parameters distributed with the CHARMM36m force field [6]. The Velocity Verlet integrator used a timestep of 2 fs, and the temperature and pressure were maintained at 300 K and 1 bar using the V-rescale thermostat and the C-rescale barostat.

### B. RETIS and REPPTIS simulations of KCl

The interfaces (in Å) for RETIS are set to $\lambda = [4.00, 4.25, 4.50, 4.75, 5.00, 5.25, 5.50, 5.75, 6.00, 18.00]$. The interfaces (in Å) for REPPTIS are set to [4.00, 5.56, 7.11, 8.67, 10.22, 11.78, 13.33, 14.89, 16.44, 18.00].

The RETIS and REPPTIS simulations were performed with the ∞RETIS code with 4 workers. For the RETIS simulation, the $[0^-]$ and $[0^+]$ ensembles used standard shooting moves, while the other $[i^+]$ ensembles used the wire-fencing move with a subtrajectory number of 2 and high-acceptance ensembles [7]. A total of 20 000 MC moves were performed, and order parameters were evaluated every 20 fs.

For the REPPTIS simulation, a new implementation in the ∞RETIS code was used, available on GitHub [8]. In the REPPTIS settings, 50% of the moves were shooting moves

| | unit | REPPTIS-MSM | | | RETIS |
|---|---|---|---|---|---|
| $\tau_{[0^-]}$ | [#ph] | | 160.4 | (±7%) | 178.9 (±6%) |
| $\tau_{[0^+]}$ | [#ph] | Eq. 13 | 2517. | (±2%) | 2654. (±7%) |
| $\tau_{\mathcal{A},1}$ | [ns] | Eq. 19 | 0.2847 | (7%) | |
| $f_A$ | [ps$^{-1}$] | Eq. 14 | 0.0187 | (±5%) | 0.0170 (±7%) |
| $P_A(\lambda_B\|\lambda_A)$ | [–] | Eq. 7 | 0.188 | (±9%) | 0.202 (±7%) |
| $k_{\text{off}}$ | [ns$^{-1}$] | Eq. 20 | 3.51 | (±6%) | 3.43 (±2%) |

Table S3: Time-dependent properties of the KCl system as estimated by the MSM framework on REPPTIS data (from 50 000 cycles), as well as the exact RETIS values (from 20 000 cycles) that serve as a reference. Relevant equations are given. Standard errors are obtained from recursive block error analysis.

and 50% were replica exchange moves between ensemble $[i^\pm]$ and its neighbors $[(i+1)^\pm]$ or $[(i-1)^\pm]$ [9]. This simulation contains 50 000 MC moves, the timestep $\Delta t = 2$ fs with subcycle 10, meaning order parameters were evaluated 20 fs.

### C. Results and error analysis of KCl

The kinetics results on KCl dissociation are givin in Table S3.

The statistical error was calculated with the recursive block error analysis, i.e. the same approach as for the 1D potentials simulations described in the previous section.

## VII. ADDITIONAL DETAILS OF TRYPSIN-BENZAMIDINE SIMULATIONS

### A. MD settings

All MD simulations were performed using GROMACS version 2021.3 [10]. The AMBER14SB force field parameters were used for trypsin [11] and the TIP3P water model for the solvent [12]. For benzamidine, the recently developed *ad hoc* parameters of Ref. 13 were used, where the partial charges were obtained using RESP [14], the non-bonded parameters were obtained using the Antechamber package [15], and the parameters of the dihedral bond between the amidine group and benzene were fitted to a QM derived potential en-

ergy function. The force field was converted from AMBER to GROMACS format using the ParmED force field conversion tool [16]. The benzamidine molecule has a net charge $q_{\text{net}}$, as the amidine group is protonated at physiological pH ($pk_a = 11.6$, $q_{\text{net}} = +1$) [17]. The system was solvated in a cubic box, ensuring a minimum distance of 1.5 nm between periodic images. Potassium $K^+$ and chlorine $Cl^-$ ions were added to neutralize the system and to reach a physiological salt concentration of 0.15 M. The solvent content consisted of 10 590 water molecules, 19 $K^+$ ions, and 28 $Cl^-$ ions. Steepest descent energy minimization was performed until the maximum force was below 1000 kJ mol$^{-1}$ nm$^{-1}$, after which short equilibration runs in the NVT and NPT ensemble were performed for 100 ps each, where both trypsin and benzamidine heavy atoms were restrained.

The unrestrained production simulation ran for 500 ns in the NPT ensemble at 298.15 K using the Nosé-Hoover thermostat [18, 19] (coupling constant of 1 ps) and at 1 bar using the Parinello-Rahman barostat [20] (coupling constant of 5 ps and compressibility of $4.5 \times 10^{-5}$ bar$^{-1}$). A time step of 2 fs was used, where hydrogen bonds were constrained using LINCS [21].

### B. RETIS and REPPTIS simulations

The 33 interfaces are located at at $\lambda =$ [4, 4.15, 4.3, 4.45, 4.6, 4.8, 5, 5.33, 5.66, 6, 6.33, 6.66, 7, 7.25, 7.5, 7.75, 8, 8.33, 8.66, 9, 9.33, 9.66, 10, 10.5, 11, 12, 13, 14, 15, 16, 17, 18, 19] (in Å).

Order parameters were evaluated every 20 fs. Trial MC moves were set at 50 % shooting moves and 50 % replica exchange moves. During the REPPTIS simulation, the GROMACS settings were identical to those used in the the equilibrium simulations.

The REPPTIS simulation produced $N_{\text{MC}} = 628\,682$ MC moves for a total of 1.079 µs MD simulation time. Of this simulation time, 0.878 µs was performed by shooting moves (of which 0.568 µs was accepted) and 0.201 µs by replica exchange moves (automatically accepted when performed). The first $N_{\text{init}} = 100\,000$ cycles were discarded for the analysis to avoid initialization effects. An exception to this is the running estimate of the global crossing probability $P_A(\lambda_A|\lambda_B)$ in Fig. S3D, where all $N_{\text{MC}}$ paths are shown.

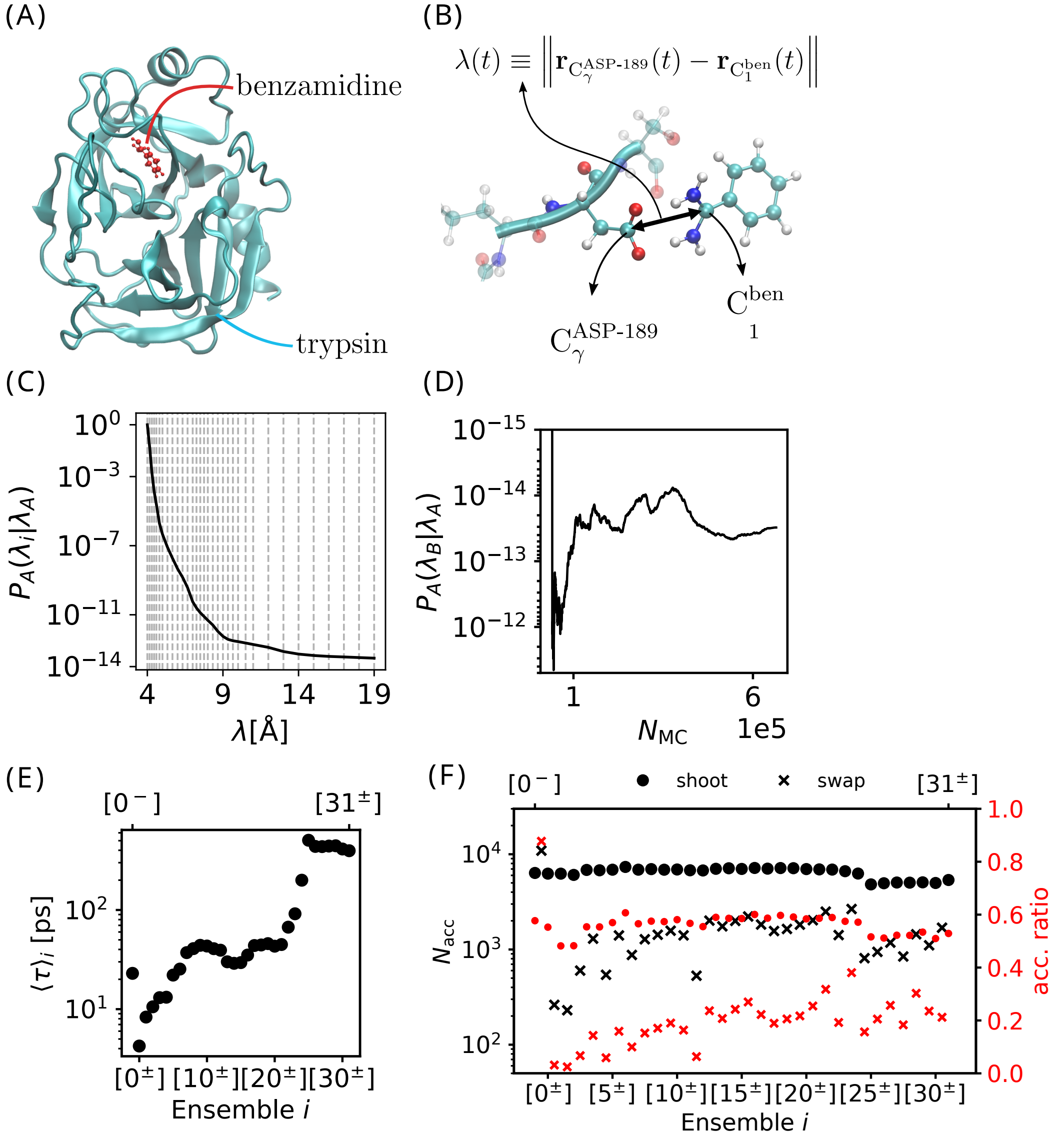


Figure S3: Panels A-B are copies of Fig. 6C and Fig. 8 in the main text. (**A**): The trypsin-benzamidine complex. (**B**): The order parameter $\lambda$ is the distance between the $\gamma$ carbon atom of ASP-189 and the amidine carbon of benzamidine. (**C**): The crossing probability profile $P_A(\lambda_i|\lambda_A)$. (**D**): The running estimate of the global crossing probability $P_A(\lambda_B|\lambda_A)$. (**E**): The average path lengths $\langle\tau\rangle_i$ of the ensembles $[0^-], [0^\pm], [1^\pm], \ldots, [31^\pm]$. (**F**): Statistics of the REPPTIS simulation with number of accepted moves $N_{\text{acc}}$ on left axis. Black dots represent the amount of accepted shooting moves in the ensembles, while black crosses represent the amount of accepted swapping moves between neighboring ensembles. In red on the right axis, the acceptance ratio $N_{\text{acc}}/N_{\text{MC}}$ of shooting (dots) and swap (crosses) trials is shown.

| | unit | | REPPTIS-MSM | | MD | |
|---|---|---|---|---|---|---|
| $\tau_{[0^-]}$ | [#ph] | | 21.4 | (±7%) | 16.3 | (±3%) |
| $\tau_{[0^+]}$ | [#ph] | Eq. 13 | 2.41 | (±3%) | 2.00 | (±1%) |
| $\tau_{\mathcal{A},1}$ | [s] | Eq. 19 | 19.3 | (±62%) | / | |
| $f_A$ | [$ps^{-1}$] | Eq. 14 | 2.10 | (±5%) | 2.74 | (±2%) |
| $P_A(\lambda_B\|\lambda_A)$ | [$10^{-14}$] | Eq. 7 | 2.47 | (±60%) | / | |
| $k_{\mathrm{off}}$ | [$s^{-1}$] | Eq. 20 | $5.17 \times 10^{-2}$ | (±61%) | / | |

Table S4: Time-dependent properties of the trypsin-benzamidine simulation as estimated by the MSM framework on REPPTIS data, and as estimated by a brute-force 500 ns MD simulation. For the latter, estimates could only be made for the flux $f_A$ and the path lengths $\tau_{[0^-]}$ and $\tau_{[0^+]}$ (in number of phase points #ph; phase points are spaced by 20 fs). Relevant MSM equations are given. Standard errors between brackets are obtained from block error analysis.

### C. Results and error analysis

The kinetic parameters of trypsin-benzamidine dissociation are given in Table S4. Here, the statistical error is substantially larger than in the other systems examined in this study. In this case, the recursive block values and the standard block values will not be identical anymore for nonlinear transformations such as MFPT calculation [3]. Consequently, the recursive block error averaging method described in the previous sections will not produce the correct error. Therefore, the first 25 000 cycles were discarded to remove the influence of the initial trajectories, and three blocks of 100 000 cycles each were constructed, from which the standard errors were computed.

The error bars on the MD values were estimated as the block average over 10 blocks.

### D. REPPTIS sampling discussion for trypsin-benzamidine

*Convergence remarks*

In comparison to KCl, the crossing probability of the trypsin-benzamidine dissociation is much more challenging to evaluate with accuracy and precision. For trypsin-benzamidine

dissociation, the crossing probability was obtained with the MSM formalism, giving a value of $P_A(\lambda_B|\lambda_A) = 2.47 \times 10^{-14} \pm 60\%$, where the error is estimated from block averaging (see section VII C). It was found to be a quantity that converges slowly. For instance, dividing the MC cycles and taking 5 blocks of 65 000 MC moves each, the resulting block values for the crossing probability range from $3 \,.\, 10^{-16}$ to $2 \,.\, 10^{-12}$, spanning 4 orders of magnitude. This indicates that 65 000 PyRETIS cycles is insufficient to make a reliable estimate. Instead, the cited $P_A(\lambda_B|\lambda_A)$ value is here the best estimate based on *all* cycles apart from the initialization cycles. To truly verify whether this estimate is a converged quantity, a further extension of the number of cycles would be required. Moreover, a reference value for the crossing probability could not be made based on RETIS, as benzamidine is trapped in metastable states making the paths prohibitively long. A reference could also not be made based on the plain MD simulation, as benzamidine did not dissociate during the 500 ns trajectory. Therefore, the REPPTIS simulation of benzamidine-trypsin showcases how our MSM offers a framework to derive a reasonable flux and rough estimate of the crossing probability from REPPTIS simulations, in those cases where RETIS and plain MD fall short.

The average path lengths of the first 10 positive ensembles are small (Fig. S3E), which is expected due to attractive forces at the binding pocket (i.e. the free energy profile has a steep slope for small $\lambda$ values). If energy barriers orthogonal to the $\lambda$ parameter are present, these small paths generated by shooting moves will likely not overcome them, resulting in the paths remaining localized near their initial trajectories. REPPTIS then depends on the replica exchange formalism to allow these ensembles to explore (more) favorable regions. The acceptance ratio for the shooting moves and replica exchange moves are shown in Fig. S3F, where the acceptance ratio of $[0^{\pm}] \leftrightarrow [1^{\pm}]$ (3.1 %) and $[1^{\pm}] \leftrightarrow [2^{\pm}]$ (2.5 %) exchange are seen to be especially low. Low swap acceptance ratios are expected for ensembles distributed over a steep free energy profile, where most paths are of type LML, providing no path overlap between adjacent ensembles required for replica exchange. This is problematic if the initial paths of these ensembles are not representative of the underlying path ensembles, where (a) the shooting move has trouble overcoming orthogonal barriers, and (b) the replica exchange move has trouble finding path overlap. As the steered MD bias was performed on the distance between the trypsin center of mass and the benzamidine center of mass rather than the distance of benzamidine to the center of the binding pocket, the initial

path might have contained a directional bias, which may have pulled benzamidine along an unfavorable dissociation pathway. While ensembles far from the bound state could relax to more favorable regions, the ensembles close to the bound state could not.

A general summary on how to assess REPPTIS convergence is provided in section VIII.

*REPPTIS kinetics in context of prior work*

The resulting dissociation rate is $k_{\text{off}} = (0.05 \pm 61\,\%)\,\text{s}^{-1}$, which is a significant underestimation of the experimental value $k_{\text{off}}^{\text{exp}} = 600\,\text{s}^{-1}$ [22] and results from other computational works [23]. This could be caused by a combination of using the steered MD trajectories as initial paths in REPPTIS and the likely hindered sampling in the ensembles close to the binding pocket, where the MC moves were unsuccessful in exploring the regions of path space relevant to the dissociation mechanism. The ∞RETIS package [24, 25] has been recently improved to provide a better generation of initial trajectories, e.g. for membrane permeation kinetics [26]. A discussion of the sampling issues is provided in section VIII, whereas a general discussion is found in Ref. 27 for the dissociation kinetics of imatinib from the ABL protein.

*Equilibrium MD validation*

As an additional validation, a 500 ns equilibrium simulation was performed to approximate the flux using standard brute force MD. In the MD, values for $\lambda$ were also calculated every 20 fs, allowing meaningful comparison with the REPPTIS result (Table S4). The MD derived flux of $2.74\,\text{ps}^{-1}$ is approximately 31 % larger than the $2.10\,\text{ps}^{-1}$ REPPTIS result, whereas the time $\tau_{[0-]}$ spent in $A$ is smaller for MD. This discrepancy can be the result of trypsin adopting a specific configuration during the equilibrium simulation with a lifetime larger than 500 ns. An estimate for the crossing probability could not be made based on plain MD, as benzamidine did not dissociate during the 500 ns trajectory. In contrast, the REPPTIS simulation of benzamidine-trypsin showcases how our MSM offers a framework to derive fluxes and rates from (RE)PPTIS simulations.

With this in mind, there clearly is a need for the REPPTIS methodology to generate

better initial paths and to better sample metastable states separated by barriers orthogonal to $\lambda$. The initial path generation is now being tackled in new versions of $\infty$RETIS [26]. A discussion of the sampling issue was presented in a recent paper [27]. While a combination of better path initialization and better choice of $\lambda$ parameter may have significantly improved sampling close to the bound state, this need remains due to biological systems often being more complex than the trypsin-benzamidine system considered here. An extension of REPPTIS to a multi-dimensional order parameter space is therefore desirable, where an enhanced free energy sampling procedure can be used to first determine relevant collective variables along the reactive pathway(s). Another possibility to tackle specifically steep energy regions is to construct a hybrid RETIS and REPPTIS methodology. RETIS-like ensembles could be positioned in the steep energy regions and connected to REPPTIS ensembles elsewhere. A methodology to exchange paths between these different ensembles should then be developed.

## VIII. ASSESSING REPPTIS CONVERGENCE

There are a few indicators for poor sampling in a REPPTIS simulation of a complex system:

1. ensembles with extremely low local crossing probabilities ($< 1\%$),

2. ensembles whose paths are extremely short, and

3. ensembles with very low acceptance ratios for the replica exchange moves.

Indicator (1) can be solved by adding more interfaces in the phase space region of the troubled ensemble. This can, however, result in indicator (2), where paths of the ensembles in this region become prohibitively short. This occurs when many paths consist of 3 phase points which blocks the exploration of phase space through inefficient shooting moves. As the end points are not a part of the ensemble (and can therefore not be used as a shooting-point), the middle phase point is reproduced in every shooting move iteration. As such, the resulting 'new' paths of a shooting move are technically a copy of the previous path. If the current path of an ensemble is in an unfavorable region of phase space, it may thus get stuck. This problem can be alleviated by the replica exchange move that can inject path segments in new regions of phase space. However, if neighboring ensembles are stuck with path types that are incompatible for replica exchange, i.e. indicator (3), then this mechanism for phase space exploration is also blocked.

All of these indicators were visible in the trypsin-benzamidine system. For example, both $[1^{\pm}]$ and $[2^{\pm}]$ ensembles were stuck with LML paths (indicator 1: no LMR means no crossing) that were extremely short (indicator 2), which results in no replica exchange between the ensembles (indicator 3).

In conclusion, if placing more interfaces does not resolve low crossing probabilities or low acceptance ratios, then it is worthwhile to investigate whether (a) the initial trajectory was generated in an unfavorable region of phase space (e.g.: large energy barriers were crossed due to directional bias forces) or (b) the order parameter does not accurately capture the

reaction mechanism.


[1] A. Ghysels, S. Roet, S. Davoudi, and T. S. van Erp, Exact non-markovian permeability from rare event simulations, Phys. Rev. Res. **3**, 033068 (2021).

[2] G. A. Huber and S. Kim, Weighted-ensemble brownian dynamics simulations for protein association reactions, Biophysical journal **70**, 97 (1996).

[3] W. Vervust, D. T. Zhang, A. Ghysels, S. Roet, T. S. van Erp, and E. Riccardi, Pyretis 3: Conquering rare and slow events without boundaries, J. Comput. Chem. **45**, 1224 (2024).

[4] D. Moroni, P. G. Bolhuis, and T. S. van Erp, Rate constants for diffusive processes by partial path sampling, J. Chem. Phys. **120**, 4055 (2004).

[5] W. L. Jorgensen, J. Chandrasekhar, J. D. Madura, R. W. Impey, and M. L. Klein, Comparison of simple potential functions for simulating liquid water, The Journal of Chemical Physics **79**, 926 (1983).

[6] J. Huang, S. Rauscher, G. Nawrocki, T. Ran, M. Feig, B. L. de Groot, H. Grubmüller, and A. D. MacKerell, CHARMM36m: an improved force field for folded and intrinsically disordered proteins, Nature Methods **14**, 71 (2017).

[7] D. T. Zhang, E. Riccardi, and T. S. van Erp, Enhanced path sampling using subtrajectory monte carlo moves, J. Chem. Phys. **158** (2023).

[8] D. Zhang, infretis: Package to perform ∞repptis (branch `infpp`), `https://github.com/dz24/infretis/tree/infpp` (2025), gitHub repository branch, accessed January 30, 2026.

[9] W. Vervust, D. T. Zhang, T. S. Van Erp, and A. Ghysels, Path sampling with memory reduction and replica exchange to reach long permeation timescales, Biophysical Journal **122**, 2960 (2023).

[10] M. J. Abraham, T. Murtola, R. Schulz, S. Páll, J. C. Smith, B. Hess, and E. Lindahl, Gromacs: High performance molecular simulations through multi-level parallelism from laptops to supercomputers, SoftwareX **1**, 19 (2015).

[11] J. A. Maier, C. Martinez, K. Kasavajhala, L. Wickstrom, K. E. Hauser, and C. Simmerling, ff14sb: improving the accuracy of protein side chain and backbone parameters from ff99sb, J. Chem. Theory Comput. **11**, 3696 (2015).

[12] W. L. Jorgensen, J. Chandrasekhar, J. D. Madura, R. W. Impey, and M. L. Klein, Comparison

of simple potential functions for simulating liquid water, J. Chem. Phys. **79**, 926 (1983).

[13] S. Raniolo and V. Limongelli, Improving small-molecule force field parameters in ligand binding studies, Front. Mol. Biosci. **8** (2021).

[14] C. I. Bayly, P. Cieplak, W. Cornell, and P. A. Kollman, A well-behaved electrostatic potential based method using charge restraints for deriving atomic charges: the RESP model, J. Phys. Chem. **97**, 10269 (1993).

[15] J. Wang, R. M. Wolf, J. W. Caldwell, P. A. Kollman, and D. A. Case, Development and testing of a general amber force field, J. Comput. Chem. **25**, 1157 (2004).

[16] M. R. Shirts, C. Klein, J. M. Swails, J. Yin, M. K. Gilson, D. L. Mobley, D. A. Case, and E. D. Zhong, Lessons learned from comparing molecular dynamics engines on the sampl5 dataset, J. Comput. Aided Mol. Des. **31**, 147 (2017).

[17] P. Y. Lam, C. G. Clark, R. Li, D. J. Pinto, M. J. Orwat, R. A. Galemmo, J. M. Fevig, C. A. Teleha, R. S. Alexander, A. M. Smallwood, *et al.*, Structure-based design of novel guanidine/benzamidine mimics: potent and orally bioavailable factor xa inhibitors as novel anticoagulants, J. Med. Chem. **46**, 4405 (2003).

[18] S. Nosé, A molecular dynamics method for simulations in the canonical ensemble, Mol. Phys. **52**, 255 (1984).

[19] W. G. Hoover, Canonical dynamics: Equilibrium phase-space distributions, Phys. Rev. A **31**, 1695 (1985).

[20] M. Parrinello and A. Rahman, Polymorphic transitions in single crystals: A new molecular dynamics method, J. Appl. Phys. **52**, 7182 (1981).

[21] B. Hess, H. Bekker, H. J. Berendsen, and J. G. Fraaije, LINCS: A linear constraint solver for molecular simulations, J. Comput. Chem. **18**, 1463 (1997).

[22] F. Guillain and D. Thusius, Use of proflavine as an indicator in temperature-jump studies of the binding of a competitive inhibitor to trypsin, Journal of the American Chemical Society **92**, 5534 (1970).

[23] F. Sohraby and A. Nunes-Alves, Advances in computational methods for ligand binding kinetics, Trends in Biochemical Sciences **48**, 437 (2023).

[24] S. Roet, D. T. Zhang, and T. S. van Erp, Exchanging replicas with unequal cost, infinitely and permanently, The Journal of Physical Chemistry A **126**, 8878 (2022).

[25] D. T. Zhang, L. Baldauf, S. Roet, A. Lervik, and T. S. van Erp, Highly parallelizable path

sampling with minimal rejections using asynchronous replica exchange and infinite swaps, Proceedings of the National Academy of Sciences **121**, e2318731121 (2024).

[26] S. Safaei, L. Baldauf, T. S. van Erp, and A. Ghysels, Exact kinetics of drug permeation using transition interface sampling, Biophys. J. (2025).

[27] W. Vervust, D. T. Zhang, E. Riccardi, T. S. van Erp, and A. Ghysels, Path sampling challenges in large biomolecular systems: RETIS and REPPTIS for ABL-imatinib kinetics, Biophys. J. (2025).
